# Supplementary material for: Auditable Unlearning for LLMs
Source: arXiv:2611.05866 source file (2026-11-04)
Supplement: Supplementary file 1 [file preview_appendix.tex]

% Standalone preview of the appendix.
%   latexmk -pdf -outdir=build figures/tikz/preview_appendix.tex   (from the repo root)
% Change the [3] to show more or fewer examples per method; drop it for all.
\documentclass[10pt]{article}
\usepackage[letterpaper,margin=1in,textwidth=5.5in]{geometry}
\usepackage{figures/tikz/dialoguebox}
\begin{document}
\appendix
\section{Qualitative examples}
\dlginputappendix[3]{figures/tikz/dialogue_appendix.tex}
\end{document}
